# Supplementary material for: SeePrivacy: Automated Contextual Privacy Policy Generation for Mobile Applications
Source: arXiv:2307.01691 source file (2023-07-09)
Supplement: Supplementary file 1 [file 10_Appendix.tex]

\section*{Appendix}

\subsection*{Manually examination of resources for CPP-related keywords list}

\noindent \textbf{How do we define ``personal identifier'' in this study?}
Personal Identifier (PID) commonly appears in data protection and privacy legislation. They have different definitions and may be further specified according to the circumstances~\cite{us_personalinfo, gdpr_personalinfo, uop_personalinfo, au_personalinfo}.
%CCPA not mentioned
%can add more later
If there is no further explanation in the legislative context, we only take the less controversial subset of common PID examples, \textit{Name}, full \textit{Date of Birthday}, \textit{Address}, \textit{Phone Number}, and \textit{Email}, to avoid the unintended comprehension.

\noindent \textbf{GDPR.~\cite{GDPR}} GDPR Personal Data: The term is defined in Art. 4 (1). Personal data are any information which are related to an identified or identifiable natural person. ``... personal data” means any information relating to an identified or identifiable natural person (‘data subject’); an identifiable natural person is one who can be identified, directly or indirectly, in particular by reference to an identifier such as a name, an identification number, location data, an online identifier or to one or more factors specific to the physical, physiological, genetic, mental, economic, cultural or social identity of that natural person; ...''

GDPR provides several examples in Recital 30 that include: Internet protocol (IP) addresses; cookie identifiers; and other identifiers such as radio frequency identification (RFID) tags.

\noindent \textbf{APP.~\cite{APP}} The explanation of personal information in APP is presented in
\footnote{https://www.oaic.gov.au/privacy/your-privacy-rights/your-personal-information/what-is-personal-information}.

\noindent \textbf{CCPA.~\cite{CCPA}} The explanation of personal information in CCPA is presented in the FAQ section
\footnote{https://oag.ca.gov/privacy/ccpa}.
